# Supplementary material for: Understanding and Mitigating Tokenization Bias in Language Models
Source: arXiv:2406.16829 source file (2024-07-05)
Supplement: Supplementary file 1 [file appendix.tex]

We want to compute the probability of the next $k$ bytes given the previous $n$ characters, where these first $n$ characters form a token $t^*_1 \in \mathcal{V}^*$, that is:
\begin{equation}
\Pr\{\bm{X}^{n+k}_{n+1}  {=} x^{n+k}_{n+1} \big{|} \bm{X}^{n}_{1}  {=} t^*_1 \} \vcentcolon= 
    \Pr\left\{(\bm{X}_{n+1}, \bm{X}_{n+2},..., \bm{X}_{n+k})  {=} (x_{n+1}, x_{n+2},..., x_{n+k}) | (\bm{X}_{1}, \bm{X}_{2},..., \bm{X}_{n})  {=} t^*_1 \right\}  
\end{equation}

Using probability marginalize rule, with the event that the the second token contains the next $k$ words or not, we have:
\begin{align}
    \Pr\{\bm{X}^{n+k}_{n+1}  {=} x^{n+k}_{n+1} \big{|} \bm{X}^{n}_{1}  {=} t^*_1 \}  &= \Pr\{\bm{X}^{n+k}_{n+1}  {=} x^{n+k}_{n+1} \big{|} \bm{T}_{1}  {=} t^*_1 \} \\
    &= \Pr\{\bm{X}^{n+k}_{n+1}  {=} x^{n+k}_{n+1}, \bm{X}^{n+k}_{n+1} \in \bm{T}_2 \big{|} \bm{T}_{1}  {=} t^*_1 \} + \Pr\{\bm{X}^{n+k}_{n+1}  {=} x^{n+k}_{n+1}, \bm{X}^{n+k}_{n+1} \notin \bm{T}_2 \big{|} \bm{T}_{1}  {=} t^*_1 \} 
\end{align}

For the first term, it is equivalent to:
\begin{align}
    \Pr\{\bm{X}^{n+k}_{n+1}  {=} x^{n+k}_{n+1}, \bm{X}^{n+k}_{n+1} \in \bm{T}_2 \big{|} \bm{T}_{1}  {=} t^*_1 \}  &= \sum_{``x^{n+k}_{n+1}\ell" \in \mathcal{V} } \Pr\{\bm{T}_{2}  {=} ``x^{n+k}_{n+1}\ell" \big{|} \bm{T}_{1}  {=} t^*_1 \} 
\end{align}
which can be easily computed with our tokenized LMs.

For the second term, we note that, under greedy prefix encoding, the following two events are equivalent:
\begin{equation}
    \{\bm{X}^{n+k}_{n+1}  {=} x^{n+k}_{n+1}, \bm{X}^{n+k}_{n+1} \notin \bm{T}_2\} \equiv \{\bm{T}_{2}  {=} t_2, \bm{X}^{n+k}_{n+j+1} {=} x^{n+k}_{n+j+1}\},
\end{equation}
where $t_2 \vcentcolon=x^{n+j}_{n+1} \in \mathcal{V}$ is a \textit{unique first token}, due to greedy encoding rule, in the string $\bm{X}^{n+k}_{n+1}$ when we know that the second token $\bm{T}_2$ is within $\bm{X}^{n+k}_{n+1}$. Then, we have:
\begin{align}
    \Pr\{\bm{X}^{n+k}_{n+1}  {=} x^{n+k}_{n+1}, \bm{X}^{n+k}_{n+1} \notin \bm{T}_2\ \big{|} \bm{T}_{1}  {=} t^*_1 \} &= \Pr \{\bm{T}_{2}  {=} t_2, \bm{X}^{n+k}_{n+j+1} {=} x^{n+k}_{n+j+1} \big{|} \bm{T}_{1}  {=} t^*_1 \} \\
    &= \Pr \{\bm{T}_2{=} t_2 \big{|} \bm{T}_{1}  {=} t^*_1 \} \Pr \{ \bm{X}^{n+k}_{n+j+1} {=} x^{n+k}_{n+j+1}\big{|}  \bm{T}_{1}  {=} t^*_1, \bm{T}_2{=} t_2 \}
\end{align}

Proceed similarly to previous steps, we have:
\begin{align}
    \Pr \{ \bm{X}^{n+k}_{n+j+1} {=} x^{n+k}_{n+j+1} \big{|} \bm{T}_2{=} t_2,  \bm{T}_{1}  {=} t^*_1 \} {=} \Pr \{ \bm{X}^{n+k}_{n+j+1} {=} x^{n+k}_{n+j+1}, \bm{X}^{n+k}_{n+j+1} \in \bm{T}_3 \big{|} \bm{T}_{1}  {=} t^*_1, \bm{T}_2{=} t_2 \}\\
    + \Pr \{ \bm{X}^{n+k}_{n+j+1} {=} x^{n+k}_{n+j+1}, \bm{X}^{n+k}_{n+j+1} \notin \bm{T}_3 \big{|} \bm{T}_{1}  {=} t^*_1, \bm{T}_2{=} t_2 \}
\end{align}

By induction, we have: 
\begin{align}
    \Pr \{ \bm{X}^{n+k}_{n+j+1} {=} x^{n+k}_{n+j+1} \big{|} \bm{T}_2{=} t_2,  \bm{T}_{1}  {=} t^*_1 \} {=} \Pr \{ \bm{X}^{n+k}_{n+j+1} {=} x^{n+k}_{n+j+1}, \bm{X}^{n+k}_{n+j+1} \in \bm{T}_3 \big{|} \bm{T}_2{=} t_2,  \bm{T}_{1}  {=} t^*_1 \}\\
    + \Pr \{ \bm{X}^{n+k}_{n+j+1} {=} x^{n+k}_{n+j+1}, \bm{X}^{n+k}_{n+j+1} \notin \bm{T}_3 \big{|} \bm{T}_2{=} t_2,  \bm{T}_{1}  {=} t^*_1 \}
\end{align}
